# Supplementary material for: Positive feedback produces broad distributions in maximum activation attained within a narrow time window in stochastic biochemical reactions
Source: arXiv:1212.1715 source file (2012-12-08)
Supplement: Supplementary file 1 [file evd_web_supp.pdf]

**Supplementary Material:**

We consider a simple chemical reaction, $C \underset{k_{-1}}{\overset{(k_1, k_p)}{\rightleftarrows}} C^*$ to calculate distributions of the maximum value of concentration of the activated species C* attained in a time interval of [0,T]. C* is produced from C with two different processes: (i) A linear first order reaction where C* is produced with a constant rate, $k_1$. (ii) C* is produced with a positive feedback where the rate ($k_p$[C*]) is proportional to the concentration of C*. The Master equation is then given by,

$$\frac{\partial P(n',n,t)}{\partial t} = (n'+1)[k_1 + k_p(n-1)](P(n'+1,n-1,t) + k_{-1}(n+1)P(n'-1,n+1,t)$$
$$-(k_1 n' + k_{-1} n + k_p n' n)P(n',n,t) \tag{1}$$

$P(n',n,t) \equiv$ Probability of having $n'$ and $n$ numbers of C and C* molecules, respectively, at any time, $t$, starting from an initial condition, $P(n',n,0) \equiv \delta_{n',N_0-m}\delta_{n,m}$.

The total number of molecules is conserved, i.e., $n' + n = N_0$. $k_{-1}$ describes the rate at which C* is converted back to C. The above equation can be also written in the following form,

$$\frac{\partial P(n,t)}{\partial t} = (N_0 - n + 1)(k_1 + k_p(n-1))P(n-1,t) + k_{-1}(n+1)P(n+1,t)$$
$$-(k_1(N_0 - n) + k_{-1}n + k_p n(N_0 - n))P(n,t) \tag{2}$$

where, $P(n,t)$ describes the probability of having n number of C* molecules at time $t$ starting from a probability distribution, $P(m,0)$ at $t$=0.

**Calculation of Extreme value distributions:**

We use the renewal equation to calculate extreme value distributions. The renewal equation is given by,

$$P(n,t|m,0) = Q_N(n,t|m,0) + \int_0^t dt'\, F_N(t'|m,0)P(n,t|N,t') \tag{3}$$

In the above equation, $Q_N(n,t|m,0)$ describes the probability of having $n$ molecules of C* species at time $t$, when an absorbing boundary condition, $Q_N(n,t|m,0) = 0$, for $n \geq N$ is imposed. $F_N(t|m,0)$ denotes the probability of arriving at the state, $n$=$N$, at time $t$ for the first time. Therefore, the probability of the number of C* reaching a maximum value $N$ at time $t$ in the time interval, [0,T], when the reaction starts with $m$ number of C* molecules at time $t$=0, is given by

$$E_N(T,t|m,0) \propto \sum_{n=0}^{N} F_N(t|m,0)Q_{N+1}(n,T|N,t) \tag{4}$$

***A. Irreversible reactions*:**

When C is converted irreversibly to C*, i.e., $k_{-1}$=0, then, $P(n,t|m,0)=0$ when $m>n$. In this limit, $E_N(T,t|m,0)$ is easier to calculate analytically, as $Q_{N+1}(N,T|m,0)=P(N,T|m,0)\quad \text{where } m\le N$.

Therefore,

$$E_N(T,t|m,0)\propto F_N(t|m,0)P(N,T|N,t) \tag{5}$$

The first passage time distribution, $F_N(t|m,0)$, can be calculated from the relation below that follows from Eq. (3), as $Q_N(N,T|m,0)=0$.

$$P(N,t|m,0)=\int_0^t dt'\, F_N(t'|m,0)P(N,t|N,t')=\int_0^t dt'\, F_N(t'|m,0)P(N,t-t'|N,0) \tag{6}$$

Using Laplace transformation for the time variables on both sides of the above equation, we can calculate the Laplace transformed first passage time distribution,

$$F_N(s|m)=\frac{P(N,s|m,0)}{P(N,s|N,0)} \tag{7}$$

We now consider two different cases to study the role of the positive feedback.

I. *Linear Model*:

We now calculate the extreme value distribution, $E_N(T, t\,|m,0)$ for the reaction in the absence of the feedback or $k_p$=0. The Master equation is given by,

$$\frac{\partial P(n',n,t)}{\partial t}=k_1(n'+1)P(n'+1,n-1,t)-k_1n'P(n',n,t) \tag{8}$$

with the initial condition,

$P(n',n,0)=\delta_{n',N_0-m}\delta_{n,m}$.

The above equation can be solved exactly using a generating function,

$F(z_1,z_2,t)=\sum_{n'=0}^{N_0}\sum_{n=0,\,n'+n=N_0}^{N_0} z_1^{n'}z_2^{n}P(n',n,t)$, which follows the equation below:

$$\frac{\partial F}{\partial t}=(z_2-z_1)\left(k_1\frac{\partial F}{\partial z_1}\right) \tag{9}$$

The above equation can be solved by method of characteristics and the resulting solution is

$$P(n',N,t|N_0-m,m,0)=P(N,t|m,0)={}^{N_0-m}C_{N_0-N}\,e^{-(N_0-N)k_1t}(1-e^{-k_1t})^{N-m} \quad (10)$$

and

$$P(N,t|N,0)=e^{-(N_0-N)k_1t}. \quad (11)$$

The Laplace transforms of Eqs.10-11 are,

$$P(N,s|m,0)={}^{N_0-m}C_{N_0-N}\int_0^\infty dt\; e^{-st}e^{-(N_0-N)k_1t}(1-e^{-k_1t})^{N-m}$$

$$={}^{N_0-m}C_{N_0-N}k_1^{-1}\int_0^1 dy(1-y)^{s/k_1+(N_0-N)-1}y^{N-m}=\frac{k_1^{-1}\;{}^{N_0-m}C_{N_0-N}\Gamma(s/k_1+N_0-N)\Gamma(N-m+1)}{\Gamma(s/k_1+N_0-m+1)} \quad (12)$$

and,

$$P(N,s|N,0)=\int_0^\infty dt\; e^{-st}e^{-(N_0-N)k_1t}=\frac{k_1^{-1}}{(s/k_1+N_0-N)} \quad (13)$$

, respectively.

Thus,

$$F_N(s|m)=\frac{P(N,s|m,0)}{P(N,s|N,0)}=\frac{(s/k_1+N_0-N)\;{}^{N_0-m}C_{N_0-N}\Gamma(s/k_1+N_0-N)\Gamma(N-m+1)}{\Gamma(s/k_1+N_0-m+1)}$$

$$=\frac{{}^{N_0-m}C_{N_0-(N-1)}\left[(N_0-N+1)/(N-m)\right]\Gamma(s/k_1+N_0-(N-1))(N-m)\Gamma((N-1)-m+1)}{\Gamma(s/k_1+N_0-m+1)}$$

$$=(N_0-N+1)k_1P(N-1,s|m,0) \quad (14)$$

The joint probability distribution is given by,

$$E_N(T,t|m,0)\propto(N_0-N+1)P(N-1,t|m,0)P(N,T|N,t) \quad (15)$$

Therefore, the un-normalized distribution of the maximum number of C* created in the time interval [0,T] is,

$$P_{\max}(N)=\int_0^T dt\; E_N(T,t|m,0)\propto(N_0-N+1)\int_0^T dt\; P(N-1,t|m,0)P(N,T|N,t)$$

$$=(N_0-N+1)e^{-k_1(N_0-N)T}\;{}^{N_0-m}C_{N_0-(N-1)}\int_0^T dt\; e^{-k_1(N_0-N+1)t}(1-e^{-k_1t})^{N-1-m}e^{k_1(N_0-N)t}$$

$$=(N_0-N+1)e^{-k_1(N_0-N)T}\;{}^{N_0-m}C_{N_0-(N-1)}\int_0^{y_T} dy y^{N-1-m}\text{ , where, } y_T=1-e^{-k_1T}$$

$$={}^{N_0-m}C_{N_0-N}e^{-k_1(N_0-N)T}(1-e^{-k_1T})^{N-m}=P(N,T|m,0) \quad (16)$$

We now calculate the average and the variance ($\sigma^2$) of $N$ from $P_{\max}(N)$.

$$P_{\max}(N) = {}^{N_0-m}C_{N_0-N} e^{-k_1(N_0-N)T}(1-e^{-k_1T})^{N-m} = {}^{N_0-m}C_{N-m} e^{-k_1(N_0-N)T}(1-e^{-k_1T})^{N-m}$$

$$= {}^{N_0-m}C_{N-m} p^{N-m}(1-p)^{(N_0-N)} \tag{17}$$

where, $p = 1-e^{-k_1T}$. Therefore,

$$\langle N-m\rangle = (N_0-m)p \Rightarrow \langle N\rangle = m+(N_0-m)p$$

and,

$$\langle (N-m)^2\rangle - \langle N-m\rangle^2 = (N_0-m)p(1-p) \Rightarrow \langle N^2\rangle - \langle N\rangle^2 = (N_0-m)p(1-p) = \sigma^2$$

The Fano factor ($f$),

$$f = \frac{\sigma^2}{\langle N\rangle} = \frac{1-p}{(m/((N_0-m)p)+1)} = \frac{e^{-k_1T}}{(m/((N_0-m)(1-e^{-k_1T}))+1)} \xrightarrow{k_1T\gg 1} e^{-k_1T}(N_0-m)/N_0 \ .$$

(18)

Therefore, the Fano factor, $f \le 1$, at any time.

The distribution of the time $t$ when the maximum value was reached is given by,

$$P_{\max}(T,t) = \sum_{N=m+1}^{N_0} E_N(T,t|m,0) \propto \sum_{N=m+1}^{N_0} (N_0-N+1)P(N-1,t|m,0)P(N,T|N,0)$$

$$= \sum_{N=m+1}^{N_0} (N_0-N+1)\,{}^{N_0-m}C_{N_0-(N-1)} e^{-k_1t} e^{-k_1(N_0-N)T}(1-e^{-k_1t})^{N-1-m}$$

$$= \sum_{N'=0}^{N_0-(m+1)} e^{-k_1t}(N_0-N'-m)\,{}^{N_0-m}C_{N_0-N'-m} e^{-k_1(N_0-(m+1)-N')T}(1-e^{-k_1t})^{N'}$$

$$= e^{-k_1t}\sum_{N'=0}^{N_0-(m+1)} (N_0-m)\ {}^{N_0-(m+1)}C_{N'} e^{-k_1(N_0-(m+1)-N)T}(1-e^{-k_1t})^{N'}$$

$$= (N_0-m)e^{-k_1t}\left(1+e^{-k_1T}-e^{-k_1t}\right)^{N_0-(m+1)}$$

(19)

<u>*Large $N_0$ results*</u>:

In the limit, $N_0 \to \infty$ and $k_1N_0 \to \tilde{k}_1$ the kinetics of the system can be well approximated by,

$$\frac{\partial P(n,t)}{\partial t} = \tilde{k}_1 P(n-1,t) - \tilde{k}_1 P(n,t)$$

(20)

For an initial condition,

$$P(n,0) = \delta_{n,m}$$

the probability distribution is given by,

$$P(n,t|m,0) = e^{-(\bar{n}-m)} \frac{(\bar{n}-m)^{n-m}}{(n-m)!} \tag{21}$$

where,

$\bar{n} = m + \tilde{k}_1 t$

The first passage time distribution is given by,

$$F_N(s|m) = \tilde{k}_1 P(N-1,\ s) \tag{22}$$

Therefore, the joint probability distribution is given by,

$$E_N(T,t|m,0) \propto P(N-1,t|m,0)P(N,T|N,t) = e^{-\tilde{k}_1 t} \frac{\left(\tilde{k}_1 t\right)^{N-1-m}}{(N-1-m)!} e^{-\tilde{k}_1 (T-t)} = e^{-\tilde{k}_1 T} \frac{\left(\tilde{k}_1 t\right)^{N-1-m}}{(N-1-m)!} \tag{23}$$

$$\therefore\ P_{\max}(N) \propto e^{-\tilde{k}_1 T} \int_0^T dt \frac{\left(\tilde{k}_1 t\right)^{N-1-m}}{(N-1-m)!} = \tilde{k}_1^{N-1-m} \frac{e^{-\tilde{k}_1 T}}{(N-m)!} \left(\tilde{k}_1 T\right)^{N-m} \propto P(N,T|m,0) \tag{24}$$

Therefore, $\langle N-m \rangle = \tilde{k}_1 T \quad \Rightarrow \langle N \rangle = m + \tilde{k}_1 T$

and, $\langle (N-m)^2 \rangle - \langle N-m \rangle^2 = \tilde{k}_1 T \quad \Rightarrow \langle N^2 \rangle - \langle N \rangle^2 = \tilde{k}_1 T$.

The Fano factor, $f = \tilde{k}_1 T / (m + \tilde{k}_1 T)$, which is always less than 1 and approaches 1 at large $\tilde{k}_1 T$.

$$P_{\max}(T,t) = \sum_{N=m+1}^{\infty} e^{-\tilde{k}_1 T} \frac{\left(\tilde{k}_1 t\right)^{N-1-m}}{(N-1-m)!} = \sum_{N'=0}^{\infty} e^{-\tilde{k}_1 T} \frac{\left(\tilde{k}_1 t\right)^{N'}}{N'!} = e^{-\tilde{k}_1 (T-t)} \quad . \tag{25}$$

The normalized distribution is given by,

$$P_{\max}(T,t) = e^{-\tilde{k}_1 (T-t)} / (1 - e^{-\tilde{k}_1 T}) \quad . \tag{26}$$

The average,

$$\langle t \rangle = \int_0^T dt\ t\ P_{\max}(T,t) = \tilde{k}_1 T / (1 - e^{-\tilde{k}_1 T}) - 1$$

and

$$\langle t^2 \rangle = \int_0^T dt\ t^2\ P_{\max}(T,t) = \frac{(\tilde{k}_1 T - 1)^2 + 1}{1 - e^{-\tilde{k}_1 T}} - \frac{2e^{-\tilde{k}_1 T}}{1 - e^{-\tilde{k}_1 T}}$$

and,

$$\langle t^2 \rangle - \langle t \rangle^2 = \frac{(\tilde{k}T)^2 e^{-\tilde{k}_1 T}}{(1 - e^{-\tilde{k}_1 T})^2} + 1 = \sigma^2$$

The variance decreases with time reaching 1 at large $k_1T$, whereas, the average increases linearly with $k_1T$, therefore, the $f$ vanishes at large $k_1T$.

II. *Feedback case:*

We consider the case where only the feedback reaction is present, i.e., $k_1$=$k_{-1}$=0. The Master equation is given by,

$$\frac{\partial P(n,t)}{\partial t} = k_p(N_0 - n + 1)(n-1)P(n-1,t) - k_p n(N_0 - n)P(n,t) \tag{27}$$

The solution of the above equation can be obtained by performing Laplace transformation on both the sides. The solution is given by for an initial condition, $P(n,0) = \delta_{n,1}$ ,

$$P(N,s|1,0) = k_p^{N-1}(N-1)!\frac{\Gamma(N_0)}{\Gamma(N_0 - N + 1)}\prod_{r=1}^{N}\frac{1}{(s + k_p r(N_0 - r))}$$
$$= \frac{k_p^{N-1}(N-1)!(N_0-1)!}{(N_0 - N)!}\prod_{r=1}^{N}\frac{1}{(s + k_p r(N_0 - r))} \tag{28}$$

and

$$P(N,t|N,0) = e^{-k_p N(N_0 - N)t} . \tag{29}$$

The first passage time distribution is given by,

$$F_N(s|m) = \frac{P(N,s|m,0)}{P(N,s|N,0)} = \frac{\frac{k_p^{N-1}(N-1)!(N_0-1)!}{(N_0 - N)!}\prod_{r=1}^{N}\frac{1}{(s + k_p r(N_0 - r))}}{1/(s + k_p N(N_0 - N))}$$
$$= k_p(N-1)(N_0 - (N-1))P(N-1,s|1,0) \tag{30}$$

Therefore,

$$E_N(T,t|m=1,0) \propto P(N-1,t|1,0)P(N,T|N,t) = k_p(N-1)(N_0 - (N-1))P(N-1,t|1,0)e^{-k_p N(N_0 - N)(T-t)} \tag{31}$$

$\therefore$

$$P_{\max}(N) = \int_0^T dt\, E_N(T,t|1,0) =$$
$$= k_p(N-1)(N_0 - (N-1))\int_0^T dt\, e^{-k_p N(N_0 - N)(T-t)}\int_{c-i\infty}^{c+i\infty} ds\, e^{st}P(N-1,s|1,0)$$
$$= k_p(N-1)(N_0 - (N-1))e^{-k_p N(N_0 - N)T}\int_{c-i\infty}^{c+i\infty} ds\, P(N-1,s|1,0)\frac{(e^{(s + k_p N(N_0 - N))T} - 1)}{s + k_p N(N_0 - N)}$$
$$= k_p(N-1)(N_0 - (N-1))\left[\int_{c-i\infty}^{c+i\infty} ds\, P(N-1,s|1,0)\frac{e^{sT}}{s + k_p N(N_0 - N)} - e^{-k_p N(N_0 - N)T}\int_{c-i\infty}^{c+i\infty} ds\, \frac{P(N-1,s|1,0)}{s + k_p N(N_0 - N)}\right]$$

Now, $\int_{c-i\infty}^{c+i\infty} ds\, \frac{P(N-1,s|1,0)}{s+k_p N(N_0-N)} = \underset{\varepsilon \longrightarrow 0}{Lt} \int_{c-i\infty}^{c+i\infty} ds\, \frac{e^{\varepsilon s} P(N-1,s|1,0)}{s+k_p N(N_0-N)} \propto P(N,\varepsilon|1,0)$

For, $N \geq 2, \quad Lt_{\varepsilon \to 0}\, P(N,\varepsilon|1,0) \longrightarrow 0$ , since, $P(N,0) = \delta_{N,1}$ .

Therefore,

$$P_{\max}(N) = k_p(N-1)(N_0-(N-1)) \int_{c-i\infty}^{c+i\infty} ds\, P(N-1,s|1,0) \frac{e^{sT}}{s+k_p N(N_0-N)} = P(N,T|1,0) \qquad (32)$$

$$P_{\max}(T,t) = \sum_{N=2}^{N_0} E_N(T,t,1) = \sum_{N=2}^{N_0} k_p(N-1)(N_0-(N-1)) P(N-1,t|1,0) e^{-k_p N(N_0-N)(T-t)} \qquad (33)$$

We evaluate $P(N,t|1,0)$ for inverting the function given in Eq. 28.

When $n < N_0/2+1/2$ ($N_0$ odd) or $n < N_0/2+1$ ($N_0$ even), then,

$$P(n,t|1,0) = \sum_{r=0}^{n-1} A_r e^{-k_p (N_0-(n-r))(n-r)t} \qquad (34)$$

where, $A_r = (1/k_p)^{n-1} \frac{(-1)^{n-1}}{r!(n-r-1)!} \frac{(N_0-2n+2r)}{(N_0-2n+r)_{r-1}(N_0-2n+r)_{n-r-1}}$

and the increasing Pochhammer symbol, $(M)_\alpha$, is defined as, $(M)_\alpha = M.(M+1)\cdots(M+\alpha) = \Gamma(M+\alpha+1)/\Gamma(M)$ .

When $N_0$ is odd, for $n \geq N_0/2+1/2$ , or, $n = (N_0+1)/2+m$ , where, $m$=0, 1, …($N_0$-1)/2,

$$P(n,t|1,0) = (k_p)^{n-1}\left[\sum_{\alpha=0}^{m} \frac{e^{-k_p(N_0-(n-\alpha))(n-\alpha)t}}{\left(\prod_{r=0,r\neq\alpha}^{m} B_{r\alpha}\right)^2 \prod_{r=2+2m}^{n-1} B_{r\alpha}} \left\{k_p t - \sum_{r=0}^{m} 2/B_{r\alpha} - \sum_{r=2+2m}^{n-1} 1/B_{r\alpha}\right\} + \sum_{\alpha=2+2m}^{n-1} \frac{e^{-k_p(N_0-(n-\alpha))(n-\alpha)t}}{\left(\prod_{r=0,}^{m} B_{r\alpha}\right)^2 \prod_{r=2+2m,r\neq\alpha}^{n-1} B_{r\alpha}}\right]$$

where, $B_{r\alpha} = (\alpha - r)(N_0 - 2n + \alpha + r)$

(35A)

When, $N_0$ is even, for $n \geq N_0/2+1$ , or, $n = N_0/2+1+m$ , where, $m$=0, 1, …$N_0$/2-1

$$P(n,t\,|\,1,0) = (k_p)^{n-1} \times \left[ \sum_{\alpha=0}^{m} \frac{e^{-k_p(N_0-(n-\alpha))(n-\alpha)t}}{\left(\prod_{\substack{r=0\\ r\neq\alpha}}^{m} B_{r\alpha}\right)^2 B_{m+1,\alpha} \prod_{r=3+2m}^{n-1} B_{r\alpha}} \left\{ k_p t - \sum_{\substack{r=0\\ r\neq\alpha}}^{m} 2/B_{r\alpha} - \sum_{r=3+2m}^{n-1} 1/B_{r\alpha} - 1/B_{m+1,\alpha} \right\} \right.$$

$$\left. + \frac{e^{-k_p(N_0-(n-(m+1)))(n-(m+1))t}}{\left(\prod_{r=0}^{m} B_{r\,m+1}\right)^2 \prod_{r=3+2m}^{n-1} B_{r\,m+1}} + \sum_{\alpha=3+2m}^{n-1} \frac{e^{-k_p(N_0-(n-\alpha))(n-\alpha)t}}{\left(\prod_{\substack{r=0\\ r\neq\alpha}}^{m} B_{r\alpha}\right)^2 B_{m+1,\alpha} \prod_{\substack{r=3+2m\\ r\neq\alpha}}^{n-1} B_{r\alpha}} \right]$$

(35B)

where, $B_{r\alpha} = (\alpha - r)(N_0 - 2n + \alpha + r)$.

*Large $N_0$ results*:

Next we consider the case, when $N_0 \to \infty$, but, $k_p N_0 = \tilde{k}_p$ is finite. The kinetics can be approximately described by a Master equation,

$$\frac{\partial P(n,t)}{\partial t} = \tilde{k}_p (n-1) P(n-1,t) - \tilde{k}_p n P(n,t) \tag{37}$$

This model was solved exactly by Max Delbruck in 1940 [1]. The solution is given by,

$$P(N,t|m,0) = \frac{m(m+1)\cdots(N-1)}{(N-m)!} (1-e^{-\tilde{k}_p t})^{N-m} e^{-\tilde{k}_p mt} \tag{38}$$

for an initial condition, $P(N,0) = \delta_{N,m}$.

The first passage time distribution,

$$F_N(s|m,0) = \tilde{k}_p (N-1) P(N-1,s|m,0) \tag{39}$$

and,

$$E_N(T,t,m) \propto P(N-1,t|m,0) P(N,T|N,t) = \tilde{k}_p (N-1) P(N-1,t|m,0) e^{-\tilde{k}_p N(T-t)} \tag{40}$$

Thus,

$$P_{\max}(N) = P(N,T|m,0) \tag{41}$$

and

$$P_{\max}(T,t)=\sum_{N=m+1}^{\infty}\tilde{k}_p(N-1)P(N-1,t|m,0)e^{-\tilde{k}_pN(T-t)}=e^{-\tilde{k}_p(T-t)}\sum_{N=m+1}^{\infty}\tilde{k}_p(N-1)P(N-1,t|m,0)e^{-\tilde{k}_p(N-1)(T-t)}$$
$$=e^{-\tilde{k}_p(T-t)}\frac{\partial}{\partial(-T)}\sum_{N=m+1}^{\infty}P(N-1,t|m,0)e^{-\tilde{k}_p(N-1)(T-t)}=e^{-\tilde{k}_p(T-t)}\frac{\partial}{\partial(-T)}\sum_{N'=m}^{\infty}P(N',t|m,0)e^{-\tilde{k}_pN'(T-t)}$$
$$=e^{-\tilde{k}_p(T-t)}\frac{\partial}{\partial(-T)}\left\langle e^{-\tilde{k}_pN(T-t)}\right\rangle \tag{42}$$

We calculate the average <exp(-$k_p N(T$-$t)$> by calculating the generating function for the above Master equation. The generating function is defined as

$$F(z,t)=\sum_{N=m}^{\infty}z^NP(N,t|m,0)$$

which satisfies the equation below,

$$\frac{\partial F}{\partial t}=\tilde{k}_pz(z-1)\frac{\partial F}{\partial z} \tag{44}$$

with the initial condition, $F(z,0)=z^m$ . The solution is given by,

$$F(z,t)=z^me^{-\tilde{k}_pmt}\left(1-(1-e^{-\tilde{k}_pt})z\right)^{-m} \tag{45}$$

The average is given by,

$$\left\langle e^{-\tilde{k}_pN(T-t)}\right\rangle=F(z,t)\big|_{z=e^{-\tilde{k}_p(T-t)}}=e^{-\tilde{k}_pm(T-t)}e^{-\tilde{k}_pmt}\left(1-(1-e^{-\tilde{k}_pt})e^{-\tilde{k}_p(T-t)}\right)^{-m}$$
$$=e^{-\tilde{k}_pmT}\left(1-(1-e^{-\tilde{k}_pt})e^{-\tilde{k}_p(T-t)}\right)^{-m} \tag{46}$$

Therefore,

$$P_{\max}(T,t)=\frac{me^{-m\tilde{k}_pT}e^{-\tilde{k}_p(T-t)}}{\left(1-(1-e^{-\tilde{k}_pt})e^{-\tilde{k}_p(T-t)}\right)^{m+1}} \tag{48}$$

**B.** ***<u>Reversible reactions:</u>***

The Master Equation can be written as,

$$\frac{\partial|P(t)\rangle}{\partial t}=L|P(t)\rangle \tag{49}$$

where, $|P(t)\rangle$ denote the column vector $\begin{pmatrix} P(0,t|m,0) \\ P(1,t|m,0) \\ \vdots \\ P(N,t|m,0) \end{pmatrix}$, and, $L$ is an operator that represents the transition matrix in the Master equation, where the elements of the matrix are given by,

$$(L)_{nn'} = (N_0 - n')(k_1 + k_p n')\delta_{n',n-1} + k_{-1}n'\delta_{n',n+1} - (k_1(N_0 - n) + k_{-1}n + k_p nn')\delta_{n',n} \quad . \quad (50)$$

We solve the above equation by numerically finding the eigenvectors and eigenvalues of the operator, $L$. Since, $L$, is a non-symmetric matrix, the right and left eigenvectors are not related by transpose and conjugation. Thus we define the right ($|R_n\rangle$) and the left eigenvectors ($\langle L_n|$), as,

$L|R_n\rangle = \lambda_n|R_n\rangle$, $\langle L_n|L = \langle L_n|\lambda_n$

where, $\langle L_n|R_m\rangle = b_n\delta_{mn}$ . Also note, $\langle L_n|L_m\rangle \neq \delta_{mn}$ or $\langle R_n|R_m\rangle \neq \delta_{mn}$, where, $|L_n\rangle$ and $\langle R_n|$ are transpose of $\langle L_n|$ and $|R_n\rangle$, respectively.

The solution of the above equation can be written as,

$$|P(t)\rangle = e^{Lt}|P(0)\rangle = \sum_{r=0}^{N_0} e^{\lambda_r t} a_r(0)|R_r\rangle = \sum_{n=0}^{N_0} a_r(t)|R_r\rangle \qquad (51)$$

where, $|P(0)\rangle$ describes the probability distribution at t=0. Therefore, $\{a_n(0)\}$ can be calculated from the initial condition, and then once the eigenvalues and eigenvectors of L are calculated, the probability distribution can be evaluated using Eq. 51. In matrix representation, the solutions can be described as below:

$\langle n|P(t)\rangle = P(n,t|m,0) = \sum_{r=0}^{N_0} e^{\lambda_r t} a_r(0) R_{rn}$ , where, $R_{rn} = \langle n|R_r\rangle$ .

The same scheme can be used to calculate the probability distribution ($Q_N(n,t|m,0)$ ) in the presence of absorbing boundary conditions. For an absorbing boundary condition, where, $Q_N(n,t|m,0) = 0$ when $n \geq N$ , the transition matrix is given by,

$(L)_{nn'} = (N_0 - n')(k_1 + k_p n')\delta_{n',n-1} + k_{-1}n'\delta_{n',n+1} - (k_1(N_0 - n) + k_{-1}n + k_p nn')\delta_{n',n}$, when, $n \leq N - 2$ .

$(L)_{nn'} = (N_0 - n')(k_1 + k_p n')\delta_{n',n-1} - (k_1(N_0 - n) + k_{-1}n + k_p nn')\delta_{n',n}$ when $n = N - 1$,

and,

$(L)_{nn'} = 0$ when, $N_0 \geq n \geq N$ . (53)

$$Q_N(n,t|m,0)=\sum_{r=0}^{N_0} e^{\lambda_r^{(N)}t} a_r^{(N)}(0) R_{rn}^{(N)} \tag{54}$$

We define the survival probability, $S_N(t|m,0)=\sum_{n=0}^{N} Q_N(n,t|m,0)=\sum_{n=0}^{N}\sum_{r=0}^{N_0} e^{\lambda_r^{(N)}t} a_r^{(N)}(0) R_{rn}^{(N)}$ .

The first passage time distribution, $F_N(t|m,0)$ , is calculated from the survival probability,

$$F_N(t|m,0)=-\frac{\partial S_N}{\partial t}=-\sum_{n=0}^{N}\sum_{r=0}^{N_0} \lambda_r^{(N)} e^{\lambda_r^{(N)}t} a_r^{(N)}(0) R_{rn}^{(N)} \tag{55}$$

The distribution of the maximal values of n for a time evolution between [0,T] is,

$$P_{\max}(N,T)=\int_0^T dt\, F_N(t|m,0) S_{N+1}(T-t|N,0)$$

$$=-\sum_{n,n'}^{N_0}\sum_{j,\,k}^{N_0} \lambda_j^{(N)} \left[\frac{e^{\lambda_j^{(N)}T}-e^{\lambda_k^{(N+1)}T}}{\lambda_j^{(N)}-\lambda_k^{(N+1)}}\right] a_j^{(N)}(0) a_k^{(N+1)}(0) R_{jn}^{(N)} R_{kn'}^{(N+1)} \tag{56}$$

and,

$$P_{\max}(T,t)=\sum_{n=m+1}^{N_0} F_n(t|m,0) S_{n+1}(T-t|n,0) \tag{57}$$


[1] M. Delbruck, J. Chem. Phys. **8**, 120 (1940).
